# Supplementary material for: Reinforcement Learning based Proactive Control for Transmission Grid Resilience to Wildfire
Source: arXiv:2107.05756 source file (2021-07-12)
Supplement: Supplementary file 1 [file appendix.tex]

\section*{Appendices}

\begin{table}[]
    \centering
    \caption{Symbol Table}
    \begin{tabular}{@{}p{0.2\columnwidth}p{0.8\columnwidth}@{}} \toprule
         \textbf{Symbol} & \textbf{Description} \\ \midrule
         $\mathcal{F}_{fire}$ & Wildfire propagation model \\
         $\mathcal{F}_{power}$ & Power system operations model \\
         $\mathcal{F}_{map}$ & Captures effect of wildfire on power system equipment \\ 
         $k$, $\Delta k$ & Time-step, step-size\\
        %  $\Delta k$ & Step size \\
         $s^{f}_{k}$ & State of wildfire at $k$ \\
         $u^{I}_{k}$, $u^{E}_{k}$ & Internal, external control input for $\mathcal{F}_{power}$ at $k$ \\
        %  $u^{E}_{k}$ & External control input for $\mathcal{F}_{power}$ at $k$ \\
         $s^{p}_{k}$ & State of power system at $k$ \\
         $X$, $x$ & Grid, cell \\
        %  $x$ & Cell \\
         $M$ & Number of cells in grid\\
         $d^{x}_{k}$ & Burning status of cell $x$ at $k$ \\
         $h^{x}_{k}$ & Amount of fuel in cell $x$ at $k$ \\
         $s^{x}_{k}$ & State of fire in a cell $x$ at $k$ \\
         $\mathcal{L}$ & Labeling function defined for $s^{x}_{k}$ \\
         $\text{C}^{x}$ & Fuel burning rate of cell $x$ \\
         $\rho^{x}_{k}$ & Probability of cell $x$ being ignited at $k$ \\
         $\text{P}^{y}_{x,k}$ & Probability of fire spreading from cell $y$ to $x$ \\
         $\mathcal{H}^{x}_{k}$ & Neighboring cells of $x$ that can contribute to fire spread to $x$ \\
         $N$ & Set of nodes or buses\\
         $T$ & Set of branches or transmission lines \\
         $z^{f}_{i}$, $z^{e}_{i}$ & Operational state of equipment (bus or branch) due to wildfire, external input \\
        %  $z^{e}_{i}$ & Operational state of equipment (bus or branch) due to external input \\
         $v^{e}_{i}$ & Selection variable for node $i$ \\
         $G_i$ & Set of cells equipment $i$ spans over \\
         $V_k$ & Set of decision variables \\
         $P^g_{i,k}$ & Power generation output at node $i$ \\
         $\Delta P^{c\_l}_{i,k}$, $\Delta P^{nc\_l}_{i,k}$ & Critical and non-critical load removed from node $i$ \\
         $\theta_{i,k}$ & Voltage angle at node $i$ \\
         $z^{o}_{i}$ & Operational state of equipment (bus or branch) due to operator action \\
         $w^{c\_l}_i$, $w^{nc\_l}_i$ & Weights associated with critical and non-critical load at node $i$ \\
         P$^{min}_i$, P$^{max}_{i}$ & Minimum and maximum power generation output at node $i$ \\
         R$^{max}_i$ & Maximum ramp rate of generating station at node $i$ \\
         $\Gamma^0$ & Very large constant \\
         $P^l_{i,k}$ & Available load demand at node $i$ in time step $k$\\
         P$^l_{i,0}$ & Initial load demand at node $i$\\
         P$^l_{0}$ & Initial system load\\
         $\alpha_i$ & Fraction of critical load at node $i$ \\
         $P^{flow}_{t,k}$ & Power flowing through line $t$ at time step $k$ \\
         P$^{maxflow}_{t}$ & Thermal power rating of line $t$ \\
         $\theta^{min}_i$, $\theta^{max}_i$ & Minimum and maximum values of voltage angles at node $i$ \\
         B$_{t}$ & Susceptance of line $t$ \\
         $q_k$ & Convergence status \\

        %  \\
        %  \textbf{ } & \textbf{RL Agent} \\
        %  \midrule
        % \Salah{need to check if we can divide into subsections (wildfire, power, agent)}
        
         $\mathcal{D}$ & Markov decision problem at hand \\
         $S$, $A$ & State and action space for $\mathcal{D}$ \\
         $\mathcal{R}$ & Reward function for $\mathcal{D}$ \\
         $r_1$, $r_2$, $r_3$, $r_4$ & Load loss, PIAW, ADIW, non-convergence  penalty \\
         $\psi^{f}_{i,k}$, $\psi^{e}_{i,k}$ & Indicates change in operational state of equipment $i$ due to wildfire, action input \\
        %  $\psi^{e}_{i,k}$ & Indicates change in operational state of equipment $i$ due to action input \\
         $\mu$ & Policy \\
         $\gamma$ & Discount factor\\ \bottomrule
    \end{tabular}
    \label{tab:symbols}
\end{table}
